# Supplementary material for: Nonadiabatic stationary behaviour in a driven low-dimensional gapped system
Source: arXiv:1402.2789 ancillary file (2014-09-24)
Supplement: Supplementary file 1 [file supplementary.pdf]

# Supplemental Material to " Nonadiabatic stationary behaviour in a driven low-dimensional gapped system"

Anna Maraga,[1] Pietro Smacchia,[1] Michele Fabrizio,[1] and Alessandro Silva[1,2]
[1]*SISSA, International School for Advanced Studies, via Bonomea 265, 34136 Trieste, Italy*
[2]*Abdus Salam ICTP, Strada Costiera 11, 34100 Trieste, Italy*

PACS numbers:

## S1. APPROACH TO THE STATIONARY STATE

In this section we discuss additional details on how the stationary state after the ramp is reached. In particular we computed the density of the excitations created, i.e., $n_{ex} = \frac{1}{L}\sum_k n_k$, with $n_k$ defined in Eq. (12), which is constant for $t > \tau$, the longitudinal magnetization of the system at the end of the ramp, i.e., $t = \tau$, and its evolution for time $t > \tau$.

As can be seen from Fig. S1(a), the number of excitations as a function of the duration of the ramp $\tau$ goes to zero as $1/\tau^2$, as expected.

Instead Fig. S1(b) shows the behavior of the magnetization measured at the end of ramp as a function of its duration. We can see that for small and large $\tau$ it approaches its equilibrium values corresponding to the initial and final transverse field respectively. In particular, Fig. S2(a) shows that the magnetization departs quadratically from its initial value, while in the limit of large $\tau$ it approaches the equilibrium value as $1/\tau$, as can be seen in Fig. S2(b). This behavior is different from the one observed for the excitation density, which decays as $1/\tau^2$, as discussed above.

Therefore, the value of the order parameter at the end of the ramp for large durations $\tau$ is very close to the equilibrium one. However, this value is not stable and it eventually decays to zero, when the ramp is stopped and the system is let evolve freely. Indeed, as we discussed in the main text, the asymptotic value of the order parameter is always zero, as long as $\tau$ is finite. As can be seen from Fig. S3(a), in which we plotted the evolution of the order parameter after the ramp, the decay to zero is always exponential. From this, one can extract a decay rate $\gamma_t$, defined in such a way that $m_x(t) \sim \exp(-\gamma_t t)$, with $t$ measuring the time after the end of the ramp. Fig. S3(b) shows the behavior of the inverse decay rate as a function of the duration of the ramp $\tau$, and in its inset we show that it grows as $\tau^2$ for large $\tau$. This shows that the asymptotic value of the magnetization is always zero, but its decay becomes slower and slower as the duration of the ramp $\tau$ is increased.

## S2. SMALL $\tau$ EXPANSION

In this section we show the derivation of the series expansion in powers of $\tau$ of the correlation length, valid for small durations of the ramp.

Introducing the variable $s = t/\tau$, which goes from 0 to 1, we write the functions $f_{1,k}$, $f_{2,k}$, and $f_{3,k}$ as power series of $\tau$, i.e.,

$$f_{1,k}(s) = \sum_{n=0}^{\infty} a_k^{(n)}(s)\,\tau^n, \tag{S1a}$$

$$f_{2,k}(s) = \sum_{n=0}^{\infty} b_k^{(n)}(s)\,\tau^n, \tag{S1b}$$

$$f_{3,k}(s) = \sum_{n=0}^{\infty} c_k^{(n)}(s)\,\tau^n, \tag{S1c}$$

with the coefficients satisfying initial conditions $a_k^{(0)}(0) = f_{1,k}(0)$, $b_k^{(0)}(0) = f_{2,k}(0)$, $c_k^{(0)}(0) = 0$, and $a_k^{(n)}(0) = b_k^{(n)}(0) = c_k^{(n)}(0) = 0$, $\forall n > 0$. Inserting the expansions in Eq. (8) of the main text, we can write down explicitly the evolution equations of the coefficients,

$$\frac{da_k^{(n+1)}}{ds} = 4\sin k\, c_k^{(n)}(s), \tag{S2a}$$

$$\frac{db_k^{(n+1)}}{ds} = 4\,(g_0 - \cos k + \Delta g\, s)\, c_k^{(n)}(s), \tag{S2b}$$

$$\frac{dc_k^{(n+1)}}{ds} = -4\,(g_0 - \cos k + \Delta g\, s)\, b_k^{(n)}(s) - 4\sin k\, a_k^{(n)}(s), \tag{S2c}$$

where we have defined $\Delta g = g_1 - g_0$. These equations can be readily integrated, obtaining an iterative procedure to compute $f_{1,k}$, $f_{2,k}$, and $f_{3,k}$ at the desired order in $\tau$. We immediately notice that, since $c_k^{(0)} = 0$, we have $a_k^{(2n+1)} = b_k^{(2n+1)} = c_k^{(2n)} = 0 \quad \forall n$, this in turn implies that the corrections to $1-2n_k$ , and so to the correlation length, with respect to the sudden quench value are given by even powers of $\tau$.

Let us compute the first non-vanishing correction. From Eq. (S2c) we derive

$$c_k^{(1)}(s) = \frac{2\Delta g\, \sin k}{\epsilon_k(0)} s^2, \tag{S3}$$

from which, using Eqs. (S2a) and (S2b),

$$a_k^{(2)}(s) = \frac{8\Delta g\, \sin^2 k}{3\epsilon_k(0)} s^3, \tag{S4}$$

$$b_k^{(2)}(s) = \frac{8\Delta g\, \sin k(g_0 - \cos k)}{3\epsilon_k(0)} s^3 + \frac{2(\Delta g)^2 \sin k}{\epsilon_k(0)} s^4. \quad \text{(S5)}$$

Using Eq.(12), we can then obtain

$$\begin{aligned} 1 - 2n_k \; &= \frac{1 + g_0 g_1 - (g_0 + g_1)\cos k}{\epsilon_k(0)\epsilon_k(1)} \\ &+ \frac{2\,(\Delta g)^2\, \sin^2 k}{3\,\epsilon_k(0)\,\epsilon_k(1)}\tau^2 + O(\tau^4). \end{aligned} \quad \text{(S6)}$$

Then, using Eq. (15), we can compute the expansion of the inverse of the correlation length up to second order in $\tau$, that is

$$\begin{aligned} \xi^{-1}(\tau) = &-\ln\left[\frac{1+g_0 g_1+\sqrt{(1-g_1^2)(1-g_0^2)}}{2}\right] \\ &-\frac{2(\Delta g)^2\left[1+g_0 g_1-\sqrt{(1-g_1^2)(1-g_0^2)}\right]}{3(g_0+g_1)^2}\tau^2 + O(\tau^4). \end{aligned} \quad \text{(S7)}$$

Finally, by inverting the previous expression, we recover Eq. (16) in the main text.

This procedure can be straightforwardly repeated for computing higher order corrections, and is easily implementable on a computer. We did it up to the eighth order in $\tau$ and we notice that all contributions are even if we exchange $g_0$ and $g_1$, that is if we either ramp up or down the transverse field.

## S3. LARGE $\tau$ EXPANSION

In this section we provide details on the derivation of the perturbative expansion in powers of $\tau$ of the correlation length, valid for large $\tau$. First, we find an approximate expression of the evolved state by applying the adiabatic perturbation theory (APT)[1]. Then we perform a power series expansion of the occupation numbers $n_k = \langle {\gamma^\tau_k}^\dagger \gamma^\tau_k \rangle_t$ in terms of the small parameter $1/\tau$ and we finally use it to compute the correlation length.

### A. Adiabatic Perturbation Theory

Our problem can be reduced to a two-level problem, greatly simplifying the general results of Ref. 1. Indeed, because of the momentum conservation, the instantaneous excited states are obtained by applying products ${\gamma^t_{-k}}^\dagger {\gamma^t_k}^\dagger$ to the ground state $|\Omega_+\rangle_t$. Since excitations to different $k$ modes are independent one from each other, we can consider the problem as a sum of independent two-level systems. Again, it is convenient to use the rescaled time $s = t/\tau$, which goes from 0 to 1. The instantaneous eigenstates of the two-level system are $|-(s)\rangle_k = (u_k(s), v_k(s))^T$ and $|+(s)\rangle_k = (v_k(s), -u_k(s))^T$, with corresponding eigenvalues $E_\pm(s) = \pm 2\epsilon_k(s)$. Using the same notation of Ref. 1, we find that the matrix elements $M_{nm}(s)$ are given by

$$M_{-+}(s) = -M_{+-}(s) = \frac{\Delta g\, \sin k}{2\epsilon_k^2(s)}, \quad \text{(S8a)}$$

$$M_{--}(s) = M_{++}(s) = 0. \quad \text{(S8b)}$$

It follows that the Berry phase $\gamma_n(s)$ and the matrix elements $W_{nm}(s)$ vanish. Moreover, the dynamical phase is such that

$$\omega_k(s) \equiv \omega_+(s) = -\omega_-(s) = \int_0^s ds'\, 2\epsilon_k(s') \quad \text{(S9)}$$

and $\Delta_{+-}(s) = -\Delta_{-+}(s) = 4\epsilon_k(s)$. Since the initial state is the ground state of the two-level system $|-(0)\rangle_k$, the initial condition is given by $b_n(0) = \delta_{n-}$.

We can now calculate explicitly corrections up to second order in the small parameter $1/\tau$. The zeroth order term in the power series expansion of APT is given by the adiabatic approximation,

$$|\psi^{(0)}(s)\rangle_k = e^{i\omega_k(s)\tau}\,|-(s)\rangle_k\,. \quad \text{(S10)}$$

The first order correction to the adiabatic approximation is

$$\begin{aligned} |\psi^{(1)}(s)\rangle_k &= e^{i\omega_k(s)\tau} b^{(1)}_{--}(s)\,|-(s)\rangle_k \\ &+ \left[e^{-i\omega_k(s)\tau} b^{(1)}_{++}(s) + e^{i\omega_k(s)\tau} b^{(1)}_{+-}(s)\right]|+(s)\rangle_k\,, \end{aligned} \quad \text{(S11)}$$

while the second order correction is

$$\begin{aligned} |\psi^{(2)}(s)\rangle_k &= \left[e^{-i\omega_k(s)\tau} b^{(2)}_{-+}(s) + e^{i\omega_k(s)\tau} b^{(2)}_{--}(s)\right]|-(s)\rangle_k \\ &+ \left[e^{i\omega_k(s)\tau} b^{(2)}_{+-}(s) + e^{-i\omega_k(s)\tau} b^{(2)}_{++}(s)\right]|+(s)\rangle_k\,. \end{aligned} \quad \text{(S12)}$$

The explicit expression of the coefficients is given below. The approximate form of the $k$ mode evolved state up to second order is

$$|\psi(s)\rangle_k = |\psi^{(0)}(s)\rangle_k + \tau^{-1}|\psi^{(1)}(s)\rangle_k + \tau^{-2}|\psi^{(2)}(s)\rangle_k + O(\tau^{-3}). \quad \text{(S13)}$$

### B. Perturbative Expansion

Using the approximate solution (S13) and noting that $\gamma^\tau_k\,|-(1)\rangle_k = 0$, which implies that at leading order $n_k(\tau) = 0$, the power series expansion of the occupation numbers up to fourth order in $1/\tau$ is

$$n_k(\tau) = \tau^{-2} n_k^{(2)}(\tau) + \tau^{-3} n_k^{(3)}(\tau) + \tau^{-4} n_k^{(4)}(\tau) + O(\tau^{-5}), \quad \text{(S14)}$$

where

$$\begin{aligned} n_k^{(2)}(\tau) &= \left|b^{(1)}_{++}(1)\right|^2 + \left|b^{(1)}_{+-}(1)\right|^2 \\ &\quad -2\cos\left(\phi_k(\tau)\right)\left[b^{(1)}_{++}(1) b^{(1)}_{+-}(1)\right], \end{aligned} \quad \text{(S15a)}$$

$$n_k^{(3)}(\tau) = 2\sin(\phi_k(\tau))\Big[ib_{+-}^{(1)}(1)b_{++}^{(2)}(1) - ib_{++}^{(1)}(1)b_{+-}^{(2)}(1)\Big], \tag{S15b}$$

$$n_k^{(4)}(\tau) \simeq \Big[b_{++}^{(2)}(1)\Big]^2 + \Big[b_{+-}^{(2)}(1)\Big]^2 + 2\cos(\phi_k(\tau))\Big[b_{++}^{(2)}(1)b_{+-}^{(2)}(1)\Big], \tag{S15c}$$

and

$$b_{++}^{(1)}(1) = \Delta g\,\frac{i\sin k}{8\,\epsilon_k^3(0)}, \tag{S16a}$$

$$b_{+-}^{(1)}(1) = -\Delta g\,\frac{i\sin k}{8\,\epsilon_k^3(1)}, \tag{S16b}$$

$$b_{++}^{(2)}(1) = (\Delta g)^2\,\frac{\sin k}{32\,\epsilon_k^3(0)}\left[\frac{3\,(g_0-\cos k)}{\epsilon_k^3(0)} + \frac{\sin^2 k}{4}\int_{g_0}^{g_1} dg\,\left(g^2-2g\cos k+1\right)^{-5/2}\right], \tag{S16c}$$

$$b_{+-}^{(2)}(1) = -(\Delta g)^2\,\frac{\sin k}{32\,\epsilon_k^3(1)}\left[\frac{3\,(g_1-\cos k)}{\epsilon_k^3(1)} - \frac{\sin^2 k}{4}\int_{g_0}^{g_1} dg\,\left(g^2-2g\cos k+1\right)^{-5/2}\right], \tag{S16d}$$

$$\phi_k(\tau) = \frac{4\tau}{\Delta g}\int_{g_0}^{g_1} dg\,\sqrt{g^2-2g\cos k+1} \tag{S16e}$$

We point out that in $n_k^{(4)}(\tau)$ we are neglecting the contribution given by ${}_k\langle\psi^{(1)}(1)|\,\gamma_k^{\tau\,\dagger}\gamma_k^{\tau}\,|\psi^{(3)}(1)\rangle_k + h.c.$, because it gives higher order corrections to the correlation length. Inserting the expansion (S14) in Eq. (15) and keeping the terms up to fourth order, we obtain

$$\xi^{-1}(\tau) = \frac{1}{\pi}\left\{\tau^{-2}\int_{-\pi}^{\pi} dk\; n_k^{(2)}(\tau) + \tau^{-3}\int_{-\pi}^{\pi} dk\; n_k^{(3)}(\tau) + \tau^{-4}\int_{-\pi}^{\pi} dk\left[n_k^{(4)}(\tau) + \left(n_k^{(2)}(\tau)\right)^2\right]\right\} + O(\tau^{-5}). \tag{S17}$$

From Eq. (S17), it is evident that oscillations in the correlation length appear as a consequence of oscillations in the occupation numbers.

Let us compute the integrals in the previous expression using Eqs. (S15) and (S16).

$$I_1 = \frac{1}{\pi}\int_{-\pi}^{\pi} dk\left[\left|b_{++}^{(1)}(1)\right|^2 + \left|b_{+-}^{(1)}(1)\right|^2\right] = (\Delta g)^2\,\frac{\left(1-g_0^2\right)^3 + \left(1-g_1^2\right)^3}{64\left(1-g_0^2\right)^3\left(1-g_1^2\right)^3}. \tag{S18}$$

$$I_2(\tau) = -\frac{2}{\pi}\int_{-\pi}^{\pi} dk\;\cos(\phi_k(\tau))\Big[b_{++}^{(1)}(1)b_{+-}^{(1)}(1)\Big] = -\frac{(\Delta g)^2}{16\pi}\,\Re\left[\int_{-\pi}^{\pi} dk\,\frac{\sin^2 k}{\left(\epsilon_k(0)\epsilon_k(1)\right)^3}\,e^{i\phi_k(\tau)}\right]. \tag{S19}$$

The contribution of the integral (S19) can be evaluated applying the stationary phase approximation. Since in the power series expansion (S17) we are keeping only terms up to fourth order, we can neglect all the contributions of $I_2(\tau)$ higher than the second order in $1/\tau$. We finally obtain

$$I_2(\tau) = -\tau^{-3/2}\,\frac{(\Delta g)^2}{64\sqrt{\pi}}\left[\frac{A_2}{C_2^{3/2}}\cos\!\left(C_0\tau + \frac{3\pi}{4}\right) + \frac{B_2}{|D_2|^{3/2}}\cos\!\left(D_0\tau - \frac{3\pi}{4}\right)\right] + O\!\left(\tau^{-5/2}\right), \tag{S20}$$

where

$$\begin{aligned}
A_2 &= \frac{1}{(1-g_0)^3(1-g_1)^3},\\
C_0 &= 2\,(2-g_0-g_1)\,,\\
C_2 &= \frac{2}{\Delta g}\left[\ln\!\left(\frac{1-g_0}{1-g_1}\right) - \Delta g\right],\\
B_2 &= \frac{1}{(1+g_0)^3(1+g_1)^3},\\
D_0 &= 2\,(2+g_0+g_1)\,,\\
D_2 &= -\frac{2}{\Delta g}\left[\ln\!\left(\frac{1+g_0}{1+g_1}\right) + \Delta g\right].
\end{aligned} \tag{S21}$$

All the other integrals containing an oscillatory part can be calculated using the stationary phase approximation. However, they give higher order corrections to the expansion (S17), so their contribution is negligible. So, the only integrals that we have to take into account are

$$I_3 = \frac{1}{\pi}\int_{-\pi}^{\pi} dk\left\{\Big[b_{++}^{(2)}(1)\Big]^2 + \Big[b_{+-}^{(2)}(1)\Big]^2\right\}, \tag{S22}$$

which has been evaluated numerically, and

$$I_4 = \frac{1}{\pi}\int_{-\pi}^{\pi} dk\left[\left|b_{++}^{(1)}(1)\right|^2 + \left|b_{+-}^{(1)}(1)\right|^2\right]^2 = \frac{3\,(\Delta g)^4}{16384}\left[\frac{1+g_0^2}{\left(1-g_0^2\right)^7} + \frac{1+g_1^2}{\left(1-g_1^2\right)^7} + \frac{2\,(1+g_0g_1)}{\left(1-g_0^2\right)\left(1-g_1^2\right)\left(1-g_0g_1\right)^5}\right]. \tag{S23}$$

Replacing the contribution of integrals $I_1$, $I_2$, $I_3$, and $I_4$ in Eq. (S17), we get an expansion of $\xi^{-1}(\tau)$ in powers of $1/\tau$:

$$\xi^{-1}(\tau) = a_2\tau^{-2} + a_3(\tau)\tau^{-7/2} + a_4\tau^{-4} + O\!\left(\tau^{-9/2}\right), \tag{S24}$$

with $a_2 = I_1$, $a_3(\tau) = I_2(\tau)\tau^{3/2}$, and $a_4 = I_3 + I_4$. Inverting this power series, we obtain the result of Eq. (17) in the main text,

$$\xi(\tau) = \frac{1}{a_2}\tau^2 + f(\tau)\sqrt{\tau} + \Lambda + O\left(\tau^{-1/2}\right). \qquad \text{(S25)}$$

with $f(\tau) = -a_3(\tau)/a_2^2$ and $\Lambda = -a_4/a_2^2$. Again, all the terms of the expansion are invariant if we exchange $g_0$ and $g_1$.

[1] G. Rigolin, G. Ortiz, and V. H. Ponce, Phys. Rev. A **78**, 052508 (2008).

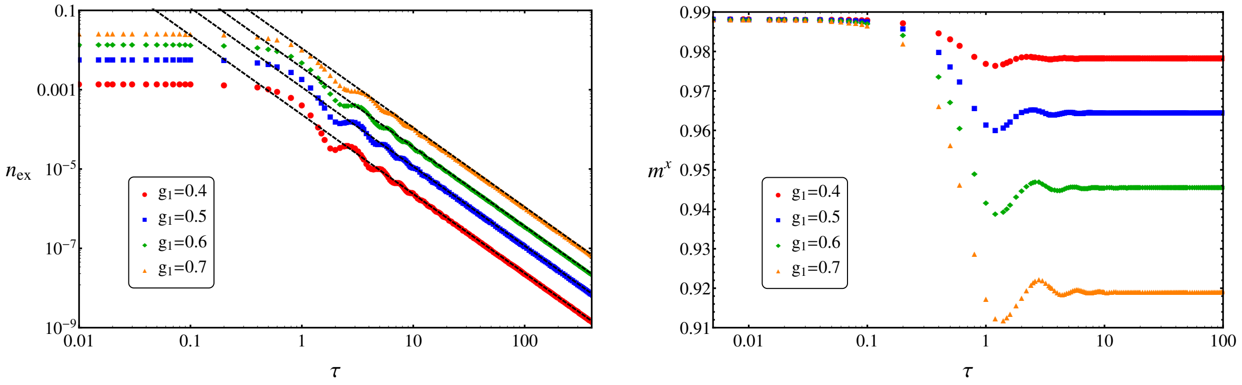


(a) (b)

Figure S1: (Color online) (a) Density of excitations $n_{ex}$ as a function of the duration of the ramp $\tau$ for ramps with $g_0 = 0.3$. The dashed lines are $\sim 1/\tau^2$ fits. (b) Longitudinal magnetization $m^x$ measured at the end of the ramp as a function of its duration $\tau$ for ramps with $g_0 = 0.3$.

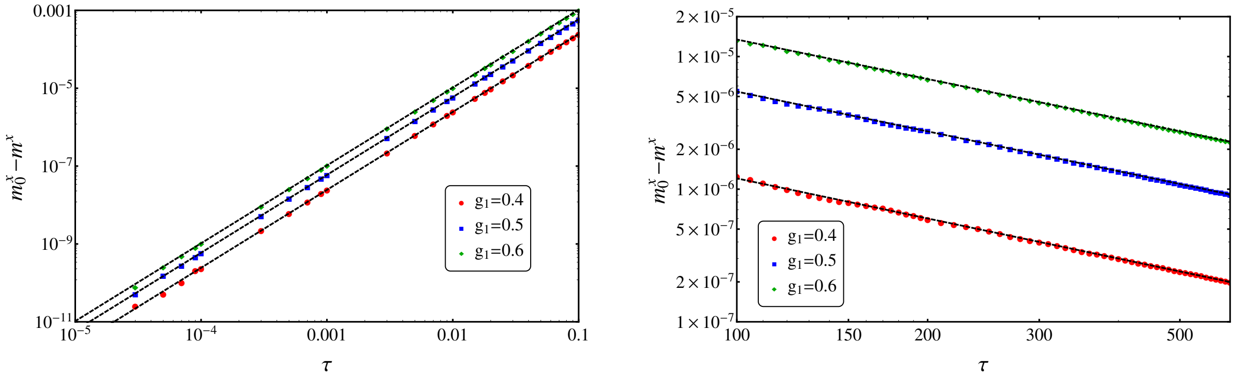


(a) (b)

Figure S2: (Color online) (a) Difference between the equilibrium value of the longitudinal magnetization $m_0^x$ corresponding to the initial value of the transverse field and its value measured at the end of the ramp $m^x$ as a function of its duration $\tau$. The initial transverse field is $g_0 = 0.3$ and the dashed lines are quadratic fits. (b) Difference between the equilibrium value of the longitudinal magnetization $m_0^x$ corresponding to the final value of the transverse field and its value measured at the end of the ramp $m^x$ as a function of its duration $\tau$. The initial transverse field is $g_0 = 0.3$ and the dashed lines are $\sim 1/\tau$ fits.

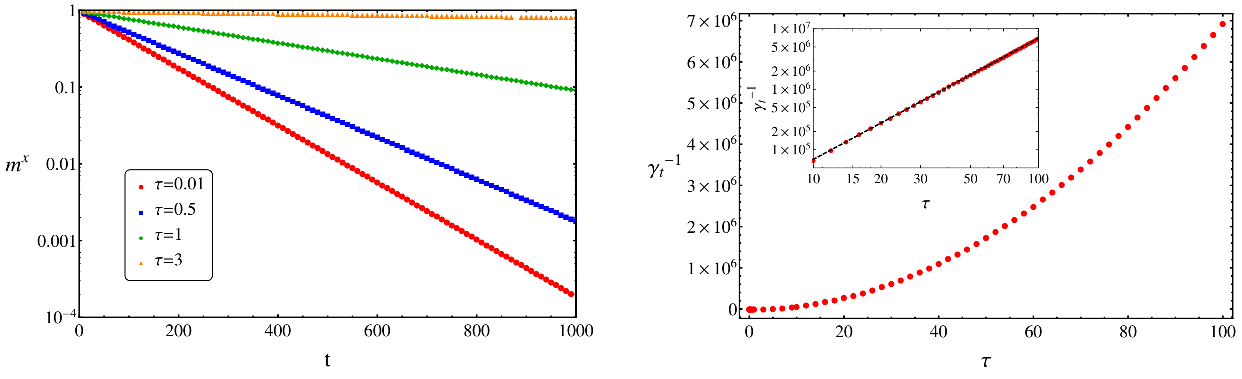


(a) (b)

Figure S3: (Color online) (a) Longitudinal magnetization $m^x$ as a function of the time $t$ elapsed after the end of the ramp in a linear-log scale for different ramp durations $\tau$. The initial and final value of the transverse field are $g_0 = 0.5$ and $g_1 = 0.2$ respectively. (b) Inverse decay rate $\gamma_t^{-1}$ as a function of the duration of the ramp $\tau$ for a ramp with $g_0 = 0.5$ and $g_1 = 0.2$. The inset shows the same plot in log-log scale with the dashed line proportional to $\tau^2$.
